# Supplementary material for: $\alpha$-$\beta$-Factorization and the Binary Case of Simon's Congruence
Source: arXiv:2306.14192 source file (2023-09-11)
Supplement: Supplementary file 1 [file appendixproofs.tex]

% Def 30
\begin{definition}
  Let \(\Omega\subseteq \Sigma\).
  We define the \emph{projection} \(\pi_\Omega : \Sigma^* \to \Omega^*\) onto \(\Omega\) as the unique morphism, such that for \(\tx\in\Sigma\) we have \(\pi_\Omega(\tx) = \tx\) if \(\tx\in\Omega\) and \(\pi_\Omega(\tx) = \varepsilon\) otherwise.
\end{definition}

\begin{remark}\label{rem:projection-preserves-sim}
Note that the projection is compatible with \(\sim_k\) in the sense that \(\pi_\Omega(w) \sim_k \pi_\Omega(\tilde w)\) if \(w \sim_k \tilde w\) because \(\ScatFact_{\leq k}(\pi_\Omega(w)) = \ScatFact_{\leq k}(w) \cap \Omega^* = \ScatFact_{\leq k}(\tilde w) \cap \Omega^* = \ScatFact(\pi_\Omega(\tilde w))\).
\end{remark}

Lastly, recall that we denote the factors according to the word's name, i.e. $\tilde{\alpha}_i\tilde{\beta}_{i+1}$ is an arch of $\tilde{w}$.

%Lemma 13
\bigskip
\ifpaper
\noindent
\textbf{\Cref{prop:simon-equiv-implies-equiv-aba-factors}.}
  Let \(w,\tilde w \in \Sigma^*\) with \(w \sim_k \tilde w\) and \(\iota(w) = \iota(\tilde w)\), then \(\ar_1^{-1}(w)\cdot w \sim_{k-1} \ar_1^{-1}(\tilde w)\cdot\tilde w\) and \(\alpha_i\beta_{i+1}\alpha_{i+1}\cdots \alpha_j \sim_{k - \iota(w) + j - i} \tilde\alpha_i\tilde\beta_{i+1}\tilde\alpha_{i+1}\cdots \tilde\alpha_j\) for all \(0 \leq i \leq j \leq \iota(w)\).
\input{proofs/simon-equiv-implies-equiv-aba-factors}
\else
\fi

\ifpaper
\bigskip

%Prop14
\noindent
\textbf{\Cref{prop:beta-equal-implies-equiv-iff-alpha-equiv}.}
  For all \(w,\tilde w\in\Sigma^*\) with \(m := \iota(w) = \iota(\tilde w) < k\) such that \(\beta_i = \tilde \beta_i\) for all \(i\in[m]\), we have \(w \sim_k \tilde{w}\) iff \(\alpha_i \sim_{k - m} \tilde\alpha_i\) for all \(i\in[m]_0\).
\input{proofs/prop-beta-equal-implies-equiv-iff-alpha-equiv}
\else
\fi

\ifpaper
\bigskip

%Theo16
\noindent
\textbf{\Cref{prop:equiv-iff-all-aba-equiv}.}
  Let \(w, \tilde w\in\Sigma^*\) with \(m \coloneqq \iota(w) = \iota(\tilde w) < k\).
  Then, \(w \sim_k \tilde w\) iff \(\alpha_{i-1}\beta_i\alpha_i \sim_{k - m + 1} \tilde\alpha_{i-1}\tilde\beta_i\tilde\alpha_i\) for all \(i\in[m]\).
\input{proofs/equiv-iff-all-aba-equiv}
\else
\fi

\ifpaper
\bigskip

%Prop 17
\noindent
\textbf{\Cref{prop:both-alpha-empty}.}
  Let \(\alpha_0 = \alpha_1 = \tilde\alpha_0 = \tilde\alpha_1 = \varepsilon\).
  Then \(w \sim_k \tilde w\) iff \(k = 1\) or \(k \geq 2\), \(\m(w) = \m(\tilde w)\), \(\w(w) = \w(\tilde w)\), and \(\core_1 \sim_k \widetilde\core_1\).
\input{proofs/both-alpha-empty.tex}
\else
\fi

\ifpaper
\bigskip

%Prop 18
\noindent
\textbf{\Cref{prop:alpha-miss-same-single}.}
  Let  \(\letters(\alpha_0) = \letters(\alpha_1) = \letters(\tilde\alpha_0) = \letters(\tilde\alpha_1) \in \binom{\Sigma}{|\Sigma|-1}\).
  We have \(w \sim_k \tilde w\) iff \(\alpha_i \sim_{k-1} \tilde\alpha_i\) for all \(i\in[1]_0\).
\input{proofs/alpha-miss-same-single}
\else
\fi

\ifpaper
\bigskip

%Prop 19
\noindent
\textbf{\Cref{prop:different-modi-force-alpha-univ-k-1}}
  Let \(w\in \Sigma^*\) with \(\iota(w) = 1\), \(k \in\mathbb N\), and \(\W \coloneqq \{ \w(\tilde w)[1] \mid \tilde w \in [w]_{\sim_k} \}\).
  If \(|\W| \geq 2\) then there exists a factorization \(\alpha_0 \eqqcolon u_1\cdots u_{k-1}\) with \(\letters(u_1) \supseteq \ldots \supseteq \letters(u_{k-1}) \supseteq \W\).
\input{proofs/different-modi-force-alpha-univ-k-1.tex}
\else
\fi

\ifpaper
\bigskip

%Prop20
\noindent
\textbf{\Cref{prop:binary:beta-alpha-cases}.}
  For all \(w\in\Sigma_2^*\), we have for all \(i\in[\iota(w)]\)
  \begin{enumerate}
    \item  \(\beta_i \in \{\ta,\tb,\ta\tb,\tb \ta\}\),
    \item  if \(\beta_i = \tx\), then \(\alpha_{i-1}, \alpha_i \in \overline \tx^+\) with $\tx \in \Sigma_2$,
    \item  if \(\beta_i = \tx\overline \tx\), then \(\alpha_{i-1} \in \tx^*\) and \(\alpha_i \in \overline \tx^*\) with $\tx \in \Sigma_2$.
  \end{enumerate}
\input{proofs/binary}
\else
\fi

\ifpaper
\bigskip

%Lemma 21
\noindent
\textbf{\Cref{prop:binary:simon-equiv-implies-beta-equiv}.}
   Let \(w,w'\in\Sigma_2^*\) with \(w \sim_k w'\) and \(m \coloneqq \iota(w) = \iota(w') < k\), then \(\m(w) = \m(w')\) and thus \(\beta_i = \beta_i'\) for all \(i\in[m]\).
\input{proofs/simon-equiv-implies-beta-equiv}
\else
\fi

\ifpaper
\bigskip

%Theo 23
\noindent
\textbf{\Cref{singleton}.}
  Let \(w \in \Sigma_2^*\), then \(|[w]_{\sim_k}| < \infty\) and in particular \(|[w]_{\sim_k}| = 1\) iff \(\iota(w) < k\) and \(|\alpha_i| < k - \iota(w)\) for all \(i\in[\iota(w)]_0\).
\input{proofs/singleton}
\else
\fi

\ifpaper
\bigskip

\noindent
\textbf{\Cref{prop:binary:simon-index-formula-per-archcount}.}
  The number of congruence classes of \(\Sigma_2^*\mathord{/}{\sim_k}\) of words with \(m < k\) arches (the entries of \Cref{tab:binary:simon-index-per-classes}) is given by
  \[
    \norm*{
    \begin{pmatrix}
            k - m & k - m & k - m \\ 
            1     & 2     & 1     \\
            k - m & k - m & k - m
    \end{pmatrix}^{\!\!m}
    \mkern-8mu\cdot
    \begin{pmatrix}
            k - m \\ 1 \\ k - m
    \end{pmatrix}
    }_1 = c_k^m
  \]
  where \(c_k^{-1} \coloneqq 1\), \(c_k^0 \coloneqq 2k + 1\), and \(c_k^m \coloneqq 2\cdot (k - m + 1) \cdot c_{k-1}^{m-1} - 2\cdot (k - m) \cdot c_{k-2}^{m-2}\).
  In the following, \(\norm{\cdot}_1\) denotes the \(1\)-norm.
\input{proofs/simon-index-formula-per-archcount}
\else
\fi

\ifpaper
\bigskip

\noindent
\textbf{\Cref{prop:ternary:same-modi-imply-equiv-iff-core-equiv}.}
Let \(\m(w) = \m(\tilde w)\) and \(\w(w) = \w(\tilde w)\), we have \(w \sim_k \tilde w\) iff \(\alpha_i \sim_{k-1} \tilde \alpha_i\) for all \(i\in[1]_0\) and \(\core_1 \sim_{k-c} \widetilde\core_1 \in \ty^*\) where \(c \coloneqq \iota(\alpha_0) + \delta_{\ty\preceq\re(\alpha_0)} + \iota(\alpha_1) + \delta_{\ty\preceq\er(\alpha_1)}\).
\ifpaper
\input{proofs/ternary-same-modi-imply-equiv-iff-core-equiv}
\else
\fi

\noindent
\textbf{\Cref{prop:ternary:beta-alpha-cases}.}
  For \(w, \tilde w \in \Sigma_3^*\) we have \(w\sim_k \tilde w\) iff \(\alpha_i\sim_{k-1} \tilde\alpha_i\) for all \(i\in[1]_0\), and
  \begin{enumerate}
    \item \(|\alphabet(\alpha_i)| = 2\), \(\alphabet(\alpha_{1-i}) \cap \alphabet(\alpha_i) = \emptyset\), and \(\iota(\alpha_i) \geq k-1\) for some \(i\in[1]_0\), or
    \item \(\m(w) = \m(\tilde w)\), \(\w(w) = \w(\tilde w)\), and \(\core \sim_{k - c} \widetilde\core\) where \(c \coloneqq \iota(\alpha_0) + \delta_{\ty\preceq \alpha_0} + \iota(\alpha_1) + \delta_{\ty \in \alpha_1}\).
  \end{enumerate}
  For all possibilities distinguishing the $\beta$, see \Cref{tab:ternary:alpha-beta-cases}.
\ifpaper
\input{proofs/ternary-beta-alpha-cases.tex}
\else
\fi
